# Supplementary material for: Learned Queries for Efficient Local Attention
Source: arXiv:2112.11435 source file (2022-04-19)
Supplement: Supplementary file 1 [file related.tex]

\section{Related}

% Please add the following required packages to your document preamble:
% \usepackage{booktabs}
\begin{table*}[]
\begin{adjustbox}{width=\textwidth}
\begin{tabular}{@{}lcccccc@{}}
\toprule
Paper & Hierarchical & Tokenization & Local Attention & Classification & Positional Encoding & Key Feature                                                                                                                                                                                                    \\ \midrule
SWIN  & \cmark          & Linear       & \cmark             & GAP            & Relative            & \begin{tabular}[c]{@{}c@{}}Shifted-Windows are used in each\\ second consecutive self-attention block\\ to capture inter-block interaction.\end{tabular}                                                       \\
HALO                      & \cmark          & Conv-Stem    & \cmark             & GAP            & Relative            & \begin{tabular}[c]{@{}c@{}}Keys and Values for each window\\ are extracted from a Halo neighbourhood\end{tabular}                                                                                              \\
CVT                       & \cmark          & Conv-Stem    & \xmark              & GAP            & N/A                 & \begin{tabular}[c]{@{}c@{}}Strided Depthwise Separable Convolutions \\ are used to extract the keys and values\\  from input features which reduces the\\  complexity of the Self-attention layer\end{tabular} \\
T2T-ViT                   & \cmark ?        & T2T          & \xmark              & CLS            & Sinusoidal          & \begin{tabular}[c]{@{}c@{}}Overlapping strided windows are reshaped \\ to form tokens which are processed via\\ linear transformers. The final tokens\\ produced are fed to ViT Backbone.\end{tabular}         \\ \bottomrule
\end{tabular}
\end{adjustbox}

\end{table*}
